# Supplementary material for: Dynamics and wetting behavior of soft particles at a fluid-fluid interface
Source: arXiv:1809.02081 ancillary file (2018-09-06)
Supplement: Supplementary file 1 [file SI.pdf]

# Supporting Information

# Dynamics and wetting behavior of soft particles at a fluid-fluid interface

Siddarth A.Vasudevan,[†] Astrid Rauh,[‡,¶] Martin Kröger,[§] Matthias Karg,[¶] and Lucio Isa[*,†]

†*Laboratory for Interfaces, Soft matter and Assembly, Department of Materials, ETH Zürich, Vladimir-Prelog-Weg 5, 8093 Zürich, Switzerland*

‡*Physical Chemistry I, University of Bayreuth, Universitätsstr. 30, 95440 Bayreuth, Germany*

¶*Physical Chemistry I, Heinrich-Heine-University, Universitätsstr. 1, 40204 Düsseldorf, Germany*

§*Polymer Physics, Department of Materials, ETH Zürich, Leopold-Ruzicka-Weg 4, 8093 Zürich, Switzerland*

E-mail: lucio.isa@mat.ethz.ch

## 1 Statistics of measured particle sizes

### 1.1 Silica core

The silica core diameters were measured from SEM images such as the ones shown in Fig. S1 using ImageJ. The mean size and standard deviation were determined by fitting the histogram of the measured particle diameters with a normal distribution function (Fig. S2). The obtained values for silica core radii are tabulated in Table 1 of the main article. The bin-size of each one of these

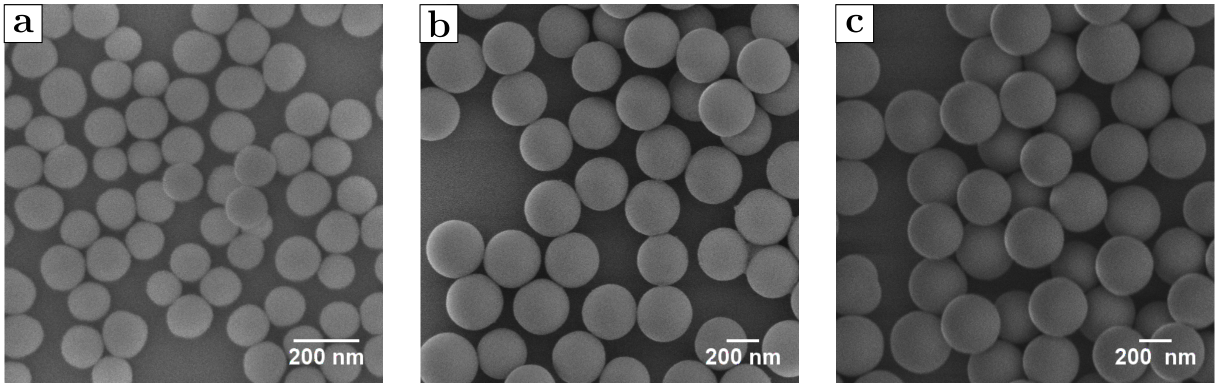


Figure S1: Representative SEM images of **(a)** C1, **(b)** C2, and **(c)** C3 silica cores.

histograms was determined by using Freedman-Diaconis rule.

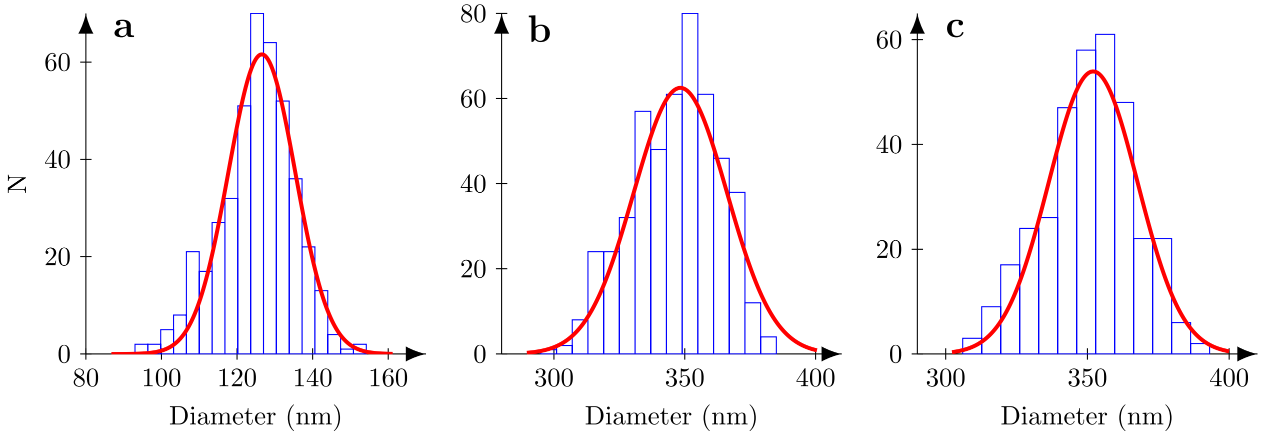


Figure S2: Histogram of measured diameters of **(a)** C1, **(b)** C2, and **(c)** C3 silica cores from SEM images.

## 1.2 C1-CSNPs

Fig. S3 shows the AFM phase images of C1-CSNPs after deposition on a silicon wafer from the water-hexane interface. Histograms of the measured interfacial diameters of C1-CSNPs from the AFM phase images are shown in Fig. S4. We note that mean size and standard deviation were not obtained by fitting the histogram with a normal distribution function but rather from the measured particle-diameter datasets. For a dataset, such as, $x = \{x_1, x_2, ..., x_n\}$, mean ($\bar{x}$) and standard deviation is equal to, respectively, $\frac{1}{n}\sum_{i=1}^{n} x_i$ and $\sqrt{\frac{1}{n-1}\sum_{i=1}^{n}(x_i - \bar{x})^2}$. Since the contrast between the polymer shell and the background is not very clear in the AFM image of the

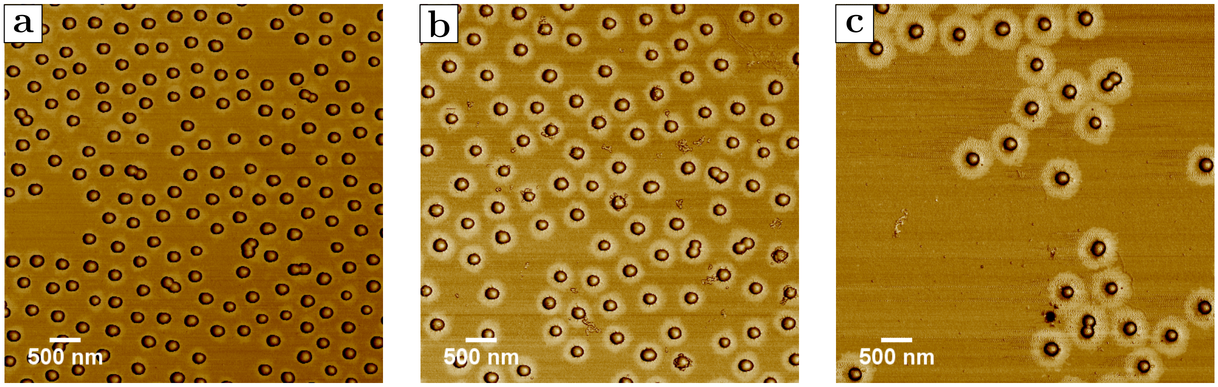


Figure S3: AFM phase images of **(a)** C1S1, **(b)** C1S2, and **(c)** C1S3 CSNPs after deposition on a silicon wafer from the water-hexane interface.

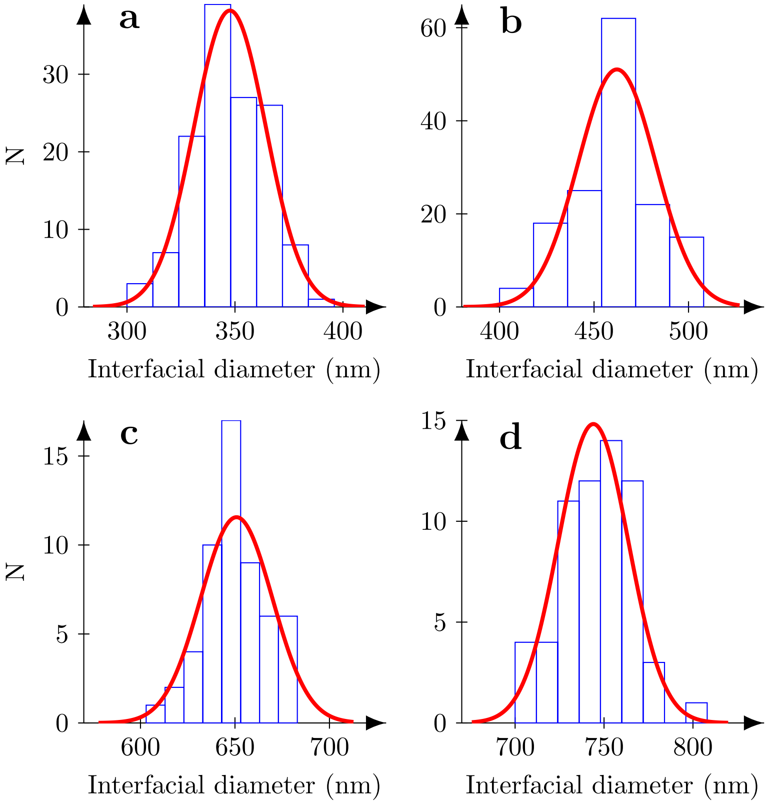


Figure S4: Histograms of the measured interfacial diameter for **(a)** C1S1, **(b)** C1S2, **(c)** C1S3, and **(d)** C1S4 CSNPs from AFM phase images. $N$ is the number count and the solid red line is a normal distribution function.

C1S1 CSNP (Fig. S3a), particle diameter obtained by fitting edge of the polymer shell with a circle leads to a underestimation of the size at the interface. Hence, we used the size obtained by fitting the histogram of the nearest-neighbor distance obtained AFM phase image of C1S1 CSNP with a normal distribution function (Fig. S5).

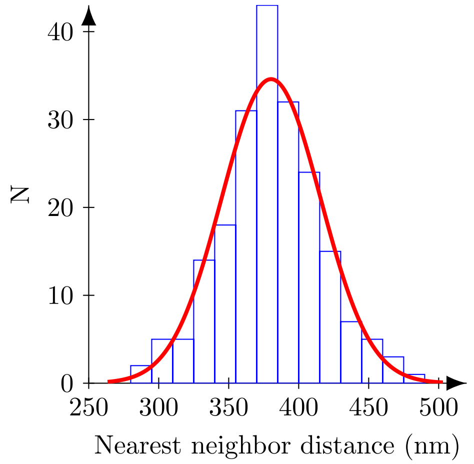


Figure S5: Histogram of nearest-neighbor distance between C1S1 CSNPs shown in Fig. S3(a). $N$ is the number count and the red solid is a fit of the data to a normal distribution.

## 1.3 C2/C3 CSNPs

Fig. S6 shows the histograms of the nearest-neighbor distance of C2-CSNPs obtained from confocal images of particle monolayers at water-hexadecane interface. The bin size is obtained by using Freedman-Diaconis rule and the red solid line is a fit of the histogram to a normal distribution, from which the mean size and standard deviation of C2-CSNPs are obtained.

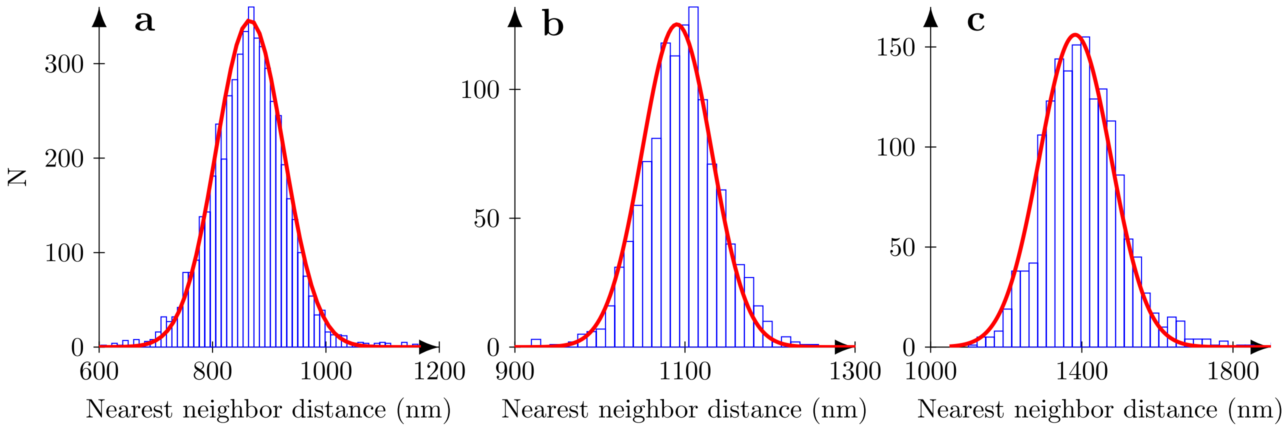


Figure S6: Histogram of the nearest-neighbor distances between **(a)** C2S1, **(b)** C2S2, and **(c)** C3S2 CSNPs in Gibbs monolayers formed at the water-hexadecane interface. $N$ is the number count and the red solid line is a fit of the histogram data to a normal distribution.
